# Supplementary material for: Local phase transitions in a model of multiplex networks with heterogeneous degrees and inter-layer coupling
Source: arXiv:1910.04466 source file (2019-10-10)
Supplement: Supplementary file 1 [file appendix.tex]

%\begin{appendices}
%\chapter{App}

%\end{appendices}
\appendix
\chapter{Algorithm to solve the maximum likelihood equations of the AOCM}
\label{A: Cost function algorithm}
In this section we propose an algorithm to (numerically) solve the maximum likelihood equations \eqref{eq: MLP equation degrees} and \eqref{eq: MLP equation overlap} for the AOCM in combination with the self consistent equation \eqref{eq: u_ij tanh equation}. We define a \textit{cost function} 
\begin{equation}
\label{eq: cost function}
C(\bm{\theta}, J) \equiv \frac{1}{2} \sum_{i=1}^N \bigg|\bigg|\overline{k}^*_i - \sum_{j=1}^Nu_{ij}^*(\theta_i,\theta_j, J) \bigg|\bigg|^2  + \frac{1}{2}\bigg|\bigg| \frac{2}{M^2}O^*  -  \sum_{i<j} \big(u_{ij}^*(\theta_i, \theta_j, J)\big)^2 \bigg|\bigg|^2
\end{equation}
where $\overline{k}^*_i$ is the desired value for the layer average degree of node $i$, $O^*$ is the desired value for the overlap of the multiplex network, and $u_{ij}^*$ is the solution to Equation \eqref{eq: u_ij tanh equation}. The value of the cost function is exactly zero for the parameter values $(\bm{\theta},J)$ that solve the maximum likelihood equations. Since the cost function is strictly positive (or zero), an approximation to the solution of the maximum likelihood equations can be found my minimizing the function. Note however that in this definition of the cost function we attributed an equal 'weight' to each maximum likelihood equation while this may not be optimal. 

An infinitesemal change in $C(\bm{\theta},J)$ is given by
\begin{equation}
\Delta C(\vec{\theta},J) \approx \sum_{k=1}^N \frac{\partial C(\vec{\theta},J)}{\partial \theta_k} \Delta \theta_k + \frac{\partial C(\vec{\theta},J)}{\partial J}\Delta J.
\end{equation}
At a given point in $(\bm{\theta},J)$ space (that is not a local minimum of $C$), taking a step in the direction of the negative gradient of $C$ moves us towards the minimum of $C$ (which we will not prove here):
\begin{equation}
\label{eq: parameters update}
\Delta \theta_k = -\eta \frac{\partial C(\vec{\theta},J)}{\partial \theta_k}, \qquad \Delta J = -\eta \frac{\partial C(\vec{\theta}, J)}{\partial J}
\end{equation}
where $\eta > 0$ controls the size of the step. We therefore need to find the derivatives $\partial C / \partial \theta_k$ and $\partial C / \partial J$:
\begin{equation}
\label{eq: C partial theta}
\frac{\partial C}{\partial \theta_k} = - \sum_{i=1}^N \bigg(\overline{k_i^*} - \sum_{j=1}^N u_{ij}^*\bigg)\sum_{j=1}^N\frac{\partial u_{ij}^*}{\partial \theta_k} - 2 \bigg(\frac{2}{M^2}O^* - \sum_{i<j}\big(u_{ij}^*\big)^2\bigg)\sum_{i<j}u_{ij}^* \frac{\partial u_{ij}^*}{\partial \theta_k}
\end{equation}
\begin{equation}
\label{eq: C partial J}
\frac{\partial C}{\partial J} = - \sum_{i=1}^N \bigg(\overline{k_i^*} - \sum_{j=1}^N u_{ij}^*\bigg)\sum_{j=1}^N\frac{\partial u_{ij}^*}{\partial J} - 2 \bigg( \frac{2}{M^2}O^* - \sum_{i<j}\big(u_{ij}^*\big)^2\bigg)\sum_{i<j}u_{ij}^* \frac{\partial u_{ij}^*}{\partial J}
\end{equation}
which require expressions for the derivatives $\partial u_{ij}^*/\partial \theta_k$ and $\partial u_{ij}^*/\partial J$. These expressions can be found implicitly by taking derivatives of both sides of the relation 
\begin{equation}
u_{ij}^* = \frac{1}{2} + \frac{1}{2}\tanh{\left(- \frac{\theta_i + \theta_j}{2} + 2Ju_{ij}^* \right)}
\end{equation}
which leads to 
\begin{equation}
\label{eq: u partial theta}
\begin{split}
\frac{\partial u_{ij}^*}{\partial \theta_k} & = \frac{1}{2}\left(1-\tanh^2{\left( -\frac{\theta_i + \theta_j}{2} + 2Ju_{ij}^* \right)} \right)\left(- \frac{\delta_i^k + \delta_j^k}{2} + 2J\frac{\partial u_{ij}^*}{\partial \theta_k} \right)
\\
& = \frac{1}{2}\left(1-(2u_{ij}^*-1)^2\right)\left( - \frac{\delta_i^k + \delta_j^k}{2} + 2J \frac{\partial u_{ij}^*}{\partial \theta_k} \right) = 
\\ 
& = -\frac{1}{4}\left(1-(2u_{ij}^*-1)^2\right)(\delta_i^k + \delta_j^k) + \left(1-(2u_{ij}^*-1)^2\right)\cdot J\frac{\partial u_{ij}^*}{\partial \theta_k}
\\
& \Rightarrow \frac{\partial u_{ij}^*}{\partial \theta_k}\cdot \left(1 -  \left(1-(2u_{ij}^*-1)^2\right)\cdot J\right) = -\frac{1}{4}\left(1 - (2u_{ij}^*-1)^2\right)(\delta_i^k + \delta_j^k) 
\\
& \Rightarrow 
\frac{\partial u_{ij}^*}{\partial \theta_k} = -\frac{\frac{1}{4}\left(1-(2u_{ij}^*-1)^2\right)(\delta_i^k + \delta_j^k)}{1 - \big[1-(2u_{ij}^*-1)^2\big]\cdot J}
= - \frac{u_{ij}^*\left(1-u_{ij}^*\right)\left(\delta_i^k + \delta_j^k\right)}{1-4Ju_{ij}^*\cdot \left(1-u_{ij}^*\right)}
\\
\end{split}
\end{equation}
and similarly 
\begin{equation}
\label{eq: u partial J}
\begin{split}
\frac{\partial u_{ij}^*}{\partial J} & =  \frac{1}{2}\left(1-(2u_{ij}^*-1)^2\right)\left( 2u_{ij}^*+ 2J \frac{\partial u_{ij}^*}{\partial J} \right) 
\\ 
& = \left(1-(2u_{ij}^*-1)^2\right)\cdot u_{ij}^* + \big[1-(2u_{ij}^*-1)^2\big]\cdot J\frac{\partial u_{ij}^*}{\partial J}
\\ 
& \Rightarrow \frac{\partial u_{ij}^*}{\partial J}\cdot \left(1 - \left(1 - (2u_{ij}^*-1)^2\right)\cdot J\right) = \left(1-(2u_{ij}^*-1)^2\right)\cdot u_{ij}^*
\\ 
& \Rightarrow 
\frac{\partial u_{ij}^*}{\partial J} = \frac{\left(1-(2u_{ij}^*-1)^2\right)\cdot u_{ij}^*}{1 - \left(1- (2u_{ij}^*-1)^2 \right)\cdot J} = \frac{4\left(u_{ij}^*\right)^2\left(1-u_{ij}^*\right)}{1-4Ju_{ij}^*\cdot \left(1-u_{ij}^*\right)}
\end{split}
\end{equation}
where we've used that $d(\tanh{x})/dx = 1-\tanh^2{x}$ and $\tanh^2[-(\theta_i + \theta_j)/2 + 2Ju_{ij}^*] = (2u_{ij}^*-1)^2$. We now have the required expressions to run the algorithm, which can be stated as
\begin{enumerate}
\item (Randomly) initialize the parameters $(\theta_1,\ldots, \theta_N, J)$
\item Solve Equation \eqref{eq: u_ij tanh equation} to obtain $u_{ij}^*$ for the current values of the parameters
\item Calculate the value of the cost function using Equation \eqref{eq: cost function}
\item Calculate the partial derivatives \eqref{eq: C partial theta} and \eqref{eq: C partial J} with the help of \eqref{eq: u partial theta} and \eqref{eq: u partial J}
\item Update the values of the parameters using Equation \eqref{eq: parameters update} 
\item Repeat starting from step 2 until a desired value of the cost function is achieved
\end{enumerate}

\noindent The downsides of this algorithm are that it may converge to a \textit{local} minimum of the cost function instead of a global minimum, which is a problem for all convex optimization algorithms. Additionally, if the value of $\eta$ is too 'large' the algorithm may not converge but if the value of $\eta$ is too 'small' the algorithm may take a very long time to run. A possible solution to this problem is to use a dynamic value of $\eta$, however we will not do that here.

\chapter{Metropolis-Hastings Algorithm}
\label{A: Metropolis-Hastings Algorithm}
In order to sample graphs from the exponential graph distribution we have made use of the \textit{Metropolis-Hastings algorithm}\cite{hastings1970monte} , which is a Markov chain Monte Carlo (MCMC) method for obtaining a sequence of random samples from a probability distribution for which direct sampling is difficult. The details of the algorithm and therefore also the knowledge required on how to correctly use the algorithm will not be discussed in this section. We will solely provide the calculations for certain quantities that are required for the implementation of the algorithm. We recommend the book "Monte Carlo Methods in Statistical Physics"\cite{newman1999monte} to gain the knowledge to properly use the algorithm and to understand its potential pitfalls.

Given the set $\mathcal{G}^M_N$ of multiplexes with $N$ nodes and $M$ layers , the algorithm attempts to move about the sample space $\mathcal{G}^M_N$ randomly in an iterative manner. Given a current sample (graph) $\vec{G} = \{g_{ij}^\alpha\} \in \mathcal{G}^M_N$, the candidate sample in the following iteration is in our case the graph that results from "flipping" a single link $g_{rs}^\gamma$ in the multiplex $\vec{G}$. We denote this mathematically as the state $F_{rs}^\gamma \vec{G}$ where $F_{rs}^\gamma$ can be seen as an operator that flips the value of $g_{rs}^\gamma$:
\begin{equation}
F_{rs}^\gamma g_{ij}^\alpha = \delta^{\gamma \alpha}_{ri,sj}(1-2g_{ij}^\alpha) + g_{ij}^\alpha
\end{equation}
where $\delta^{\gamma \alpha}_{ri,sj} \equiv \delta_{ri}\delta_{sj}\delta^{\gamma\alpha}$ is the product of three Kronecker deltas and is therefore only nonzero if $\gamma$ equals $\alpha$, $r$ equals $i$ and $s$ equals $j$ simultaneously. The proposed candidate sample is then accepted with a probability
\begin{equation}
\label{eq: Acceptance probability}
P\left[ \vec{G} \rightarrow F_{rs}^\gamma \vec{G} \right] = \min{\left\{1, e^{-\Delta H_{rs}^\gamma}\right\}}
\end{equation}
where 
\begin{equation}
\label{eq: delta H}
\Delta H_{rs}^\gamma \equiv H(F^\gamma_{rs}\vec{G}) - H(\vec{G})
\end{equation}
is the difference between the Hamiltonian of the proposed candidate graph and the current graph. The acceptance probability \eqref{eq: Acceptance probability} can be evaluated once the parameters $\theta_i$ where $i=1,\ldots, K$ of the model (see Equation \eqref{eq: ERGM Hamiltonian}) are specified. A typical implementation of the algorithm is shown in Algorithm \ref{algorithm: Metropolis} on page \pageref{algorithm: Metropolis} where $T$ is the desired number of iterations which should typically be much larger than the size of the system: $T \gg MN(N-1)/2$. 

The calculation of $\Delta H^\gamma_{rs}$ can be quite computationally intensive when calculating both $H(F^\gamma_{rs}\vec{G})$ and $H(\vec{G})$ individually. Note that the difference in the Hamiltonian can be written as a difference in the values of the graph properties $z_i(\vec{G})$ that we have chosen to constrain in the ERGM:
\begin{equation}
\label{eq: graph property difference Hamiltonian}
\Delta H^\gamma_{rs} =  \sum_{i=1}^K \theta_i z_i(F^\gamma_{rs}\vec{G}) - \sum_{i=1}^K \theta_i z_i(\vec{G}) = \sum_{i=1}^K \theta_i \left( \Delta z_i\right)^\gamma_{rs}
\end{equation}
where 
\begin{equation}
\label{eq: graph property difference}
\left(\Delta z_i\right)^\gamma_{rs} \equiv z_i(F^\gamma_{rs}\vec{G}) - z_i(\vec{G}). 
\end{equation}
In some cases it is possible to directly calculate \eqref{eq: graph property difference} which speeds up the computation considerably in comparison to calculating $z_i(F^\gamma_{rs}\vec{G})$ and $z_i(\vec{G})$ separately. The algorithm for such cases is shown in Algorithm \ref{algorithm: faster Metropolis} on page \pageref{algorithm: faster Metropolis}.

\subsection*{Direct calculations of $\Delta H^{\gamma}_{rs}$}
In this section we will demonstrate direct calculations of \eqref{eq: graph property difference} for a variety of graph properties $z(\vec{G})$ that can be chosen to be constrained in the ERGM.

\paragraph{The total number of links} In the case where $z(\vec{G})$ is the total number of links $L(\vec{G})$ we write
\begin{equation}
z(\vec{G}) = L(\vec{G}) = \sum_{i<j}\sum_{\alpha=1}^M g_{ij}^\alpha.
\end{equation}
The difference between the number of links when flipping the link $g_{rs}^{\gamma}$ is then 
\begin{equation}
\begin{split}
\left(\Delta L\right)^{\gamma}_{rs} & =  L(F^\gamma_{rs}\vec{G}) - L(\vec{G}) \\
& = \sum_{i<j}\sum_{\alpha=1}^M\left(\delta^{\gamma\alpha}_{ri,sj}(1-2g_{ij}^\alpha) + g_{ij}^\alpha \right) - \sum_{i<j}\sum_{\alpha=1}^Mg_{ij}^\alpha \\
& = 1-2g_{rs}^\gamma 
\end{split}
\end{equation}
which means that the number of links either changes by $+1$ or $-1$ depending on the initial value of $g_{rs}^\gamma$, which is exactly what one would expect. 
\paragraph{The overlap} In the case where $z(\vec{G})$ is the overlap $O$ as defined in \eqref{eq: global overlap} we write 
\begin{equation}
z_i(\vec{G}) = O(\vec{G}) = \sum_{i<j}\sum_{\alpha<\beta}g_{ij}^\alpha g_{ij}^\beta = \frac{1}{2}\sum_{i<j}\left(\sum_{\alpha}g_{ij}^\alpha \sum_{\beta}g_{ij}^\beta - \sum_{\alpha}g_{ij}^\alpha \right)
\end{equation}
The difference in the overlap when flipping the link $g_{rs}^\gamma$ is then
\begin{equation}
\begin{split}
\left(\Delta O\right)^\gamma_{rs} & = O(F^\gamma_{rs}\vec{G}) - O(\vec{G}) \\
& = \frac{1}{2}\sum_{i<j}\left(\sum_{\alpha}\left(\delta^{\gamma \alpha}_{ri,sj}(1-2g_{ij}^\alpha) + g_{ij}^\alpha \right)\sum_{\beta}\left(\delta^{\gamma \beta}_{ri,sj}(1-2g_{ij}^\beta) + g_{ij}^\beta   \right)  - \sum_{\alpha}\left(\delta^{\gamma \alpha}_{rs,sj}(1-2g_{ij}^\alpha) + g_{ij}^\alpha  \right)  \right)
\\
&  - \frac{1}{2}\sum_{i<j}\left(\sum_{\alpha}g_{ij}^\alpha \sum_{\beta}g_{ij}^\beta - \sum_{\alpha}g_{ij}^\alpha \right) 
\\ 
& = \frac{1}{2}\sum_{i<j}\Bigg( \sum_{\alpha}\left(\delta^{\gamma \alpha}_{ri,sj}(1-2g_{ij}^\alpha) \right) \sum_{\beta}\left(\delta^{\gamma\beta}_{ri,sj}(1-2g_{ij}^\beta)  \right) + \sum_{\alpha}\left(\delta^{\gamma \alpha}_{ri,sj}(1-2g_{ij}^\alpha) \right) \sum_{\beta}g_{ij}^\beta  
\\
& +  \sum_{\beta}\left(\delta^{\gamma \beta}_{ri,sj}(1-2g_{ij}^\beta) \right) \sum_{\alpha}g_{ij}^\alpha   - \sum_{\alpha}\left(\delta^{\gamma\alpha}_{ri,sj}(1-2g_{ij}^\alpha) \right)  \Bigg) 
\\
& = \frac{1}{2}\left( \left(1-2g_{rs}^\gamma\right)^2 + 2\left(1-2g_{rs}^\gamma\right)\sum_{\alpha}g_{rs}^\alpha - 1 + 2g_{rs}^\gamma \right) 
\\
& = \left(1-2g_{rs}^\gamma\right)\sum_{\alpha}g_{rs}^\alpha + g_{rs}^\gamma 
\end{split}
\end{equation}

\begin{algorithm}[H]
\label{algorithm: Metropolis}
\SetKwData{Left}{left}\SetKwData{This}{this}\SetKwData{Up}{up}
\SetKwInOut{Input}{input}\SetKwInOut{Output}{output}

 \Input{ $\theta_i, J, N, M, T$ \tcp*[f]{For $i=1,\ldots, K$}} 
 %\BlankLine
 
 %\KwResult{how to write algorithm with \LaTeX2e }
 initialization\; 
 \For{$t = 1,\ldots, T$}{
  draw a random layer $\alpha \in \{1,\ldots, M \}$\;
  draw a random pair of nodes $(i,j)$ with $i<j$\;
  calculate $\Delta H_{ij}^\alpha$ \tcp*[f]{Given by Equation \eqref{eq: delta H}} \;
  set $\textrm{Prob(accept move)} =  \min{\left\{1, e^{-\Delta H_{rs}^\gamma}\right\}} $ \;
  draw $r \in [0,1]$ \;
  \If{$r < $ \upshape Prob(accept move)}{
   set $g_{ij}^\alpha \rightarrow 1 - g_{ij}^\alpha $\;
   set $g_{ji}^\alpha \rightarrow 1 - g_{ji}^\alpha $\;
   }
 }
\caption{An example of the implementation of the Metropolis-Hastings algorithm in pseudocode}
\end{algorithm}

\begin{algorithm}[H]
\label{algorithm: faster Metropolis}
\SetKwData{Left}{left}\SetKwData{This}{this}\SetKwData{Up}{up}
\SetKwInOut{Input}{input}\SetKwInOut{Output}{output}

 \Input{ $\theta_i, J, N, M, T$ \tcp*[f]{For $i=1,\ldots, K$}} 
 \BlankLine
 initialization\; 
 calculate and save $z_i(\vec{G})$ for $i=1,\ldots, K$ \;
 \For{$t = 1,\ldots, T$}{
  draw a random layer $\alpha \in \{1,\ldots, M \}$\;
  draw a random pair of nodes $(i,j)$ with $i<j$\;
  calculate $\left(\Delta z_i\right)^\alpha_{ij}$ for $i=1,\ldots, K$ \;
  calculate $\Delta H_{ij}^\alpha$ \tcp*[f]{Given by Equation \eqref{eq: graph property difference Hamiltonian}} \;
  set $\textrm{Prob(accept move)} =  \min{\left\{1, e^{-\Delta H_{rs}^\gamma}\right\}} $ \;
  draw $r \in [0,1]$ \;
  \If{$r < $ \upshape Prob(accept move)}{
   set $g_{ij}^\alpha \rightarrow 1 - g_{ij}^\alpha $\;
   set $g_{ji}^\alpha \rightarrow 1 - g_{ji}^\alpha $\;
   set $z_i(\vec{G})\rightarrow z_i(\vec{G}) + \left(\Delta z_i\right)^\alpha_{ij}$ for $i=1, \ldots, K$ \;
   }
 }
 \caption{An example of the implementation of the Metropolis-Hastings algorithm in pseudocode using the direct calculation of $\Delta H^\alpha_{ij}$}
\end{algorithm}

\chapter{Distributions for $x_{0,i}$ used in numerical simulations}
\label{A: Distributions}
In Chapter $\ref{chapter: 4}$ we have tested the validity and accuracy of the equations obtained in Chapter $\ref{chapter: 3}$ which required sampling the $N = 100$ values for $x_{0,i}$. In this Appendix we show the histograms of the sampled data for a variety of distributions. We omit the Delta distribution which is peaked at $x_{0,i} = 0.25$ that we've used in Chapter $\ref{chapter: 4}$. We note that in the case where $x_{0,i}$ was sampled from a log-normal distribution with a relatively small value of $\sigma$, we've chosen a value for $\mu$ such that the log-normal distribution is sharply peaked around $x_{0,i} \approx 0.247$ which is approximately $0.25$ as can be seen in Figure \ref{fig:lognormal histograms}. 
\begin{figure}
\begin{center}
\includegraphics[width=.49\textwidth]{powerlaw_histogram_gamma_1}
\includegraphics[width=.49\textwidth]{powerlaw_histogram_gamma_2}
\includegraphics[width=.49\textwidth]{powerlaw_histogram_gamma_3}
\includegraphics[width=.49\textwidth]{powerlaw_histogram_gamma_4}
\end{center}
\caption{The above figure shows the histograms of the sampled values for $x_{0,i}$ which were used in the numerical simulations in Chapter \ref{chapter: 4} in the case where $x_{0,i}$ was sampled from a power-law distribution. Each plot corresponds to a different value for $\gamma$ as shown in the title.}
\label{fig:powerlaw histograms}
\end{figure}

\begin{figure}
\begin{center}
\includegraphics[width=.49\textwidth]{lognormal_histogram_sigma_0-00001}
\includegraphics[width=.49\textwidth]{lognormal_histogram_sigma_0-001}
\includegraphics[width=.49\textwidth]{lognormal_histogram_sigma_0-1}
\includegraphics[width=.49\textwidth]{lognormal_histogram_sigma_1-0}
\includegraphics[width=.49\textwidth]{lognormal_histogram_sigma_10-0}

\end{center}
\caption{The above figure shows the histograms of the sampled values for $x_{0,i}$ which were used in the numerical simulations in Chapter \ref{chapter: 4} in the case where $x_{0,i}$ was sampled from a log-normal distribution. Each plot corresponds to a different value for $\sigma$ as shown in the title}
\label{fig:lognormal histograms}
\end{figure}
